# Supplementary material for: MangaNinja: Line Art Colorization with Precise Reference Following
Source: arXiv:2501.08332 source file (2025-01-14)
Supplement: Supplementary file 1 [file appendix.tex]

\clearpage
\appendix

\setcounter{figure}{0}
\setcounter{table}{0}
\setcounter{equation}{0}
\setcounter{page}{1}
\maketitlesupplementary

The supplementary materials are structured as follows:

\begin{enumerate}[label=\textbullet, leftmargin=2em, itemsep=1em]
    \item We present and analyze additional possible solutions for reference-based line art colorization.
    \item A user study is conducted to further evaluate the superiority of our method, and a visual example is included to illustrate the benchmark we constructed for easier understanding.
    \item Extensive ablation studies are conducted, including experiments on the image feature extractor and the progressive patch shuffle training strategy.
    \item We provide more visual results of \method.
\end{enumerate}
Finally, we sincerely invite you to review the \textbf{MP4} files in our supplementary materials, which contain visualizations of the relevant results.
\tableofcontents
\section{Analysis of More Possible Solutions} 
\subsection{Analysis of line art video colorization methods}
Recent advancements~\cite{xing2024tooncrafter} are being made in video line art colorization. 
ToonCrafter~\cite{xing2024tooncrafter} is a video interpolation model that allows users to input line art as a control condition for colorization. LVCD is another video line art colorization method, enabling users to colorize a sequence based on an initial video frame and subsequent line art frames.
We explore the potential of using such video methods for image-based line art colorization.
\begin{figure}[t]
    \centering
    \includegraphics[width=1\linewidth]{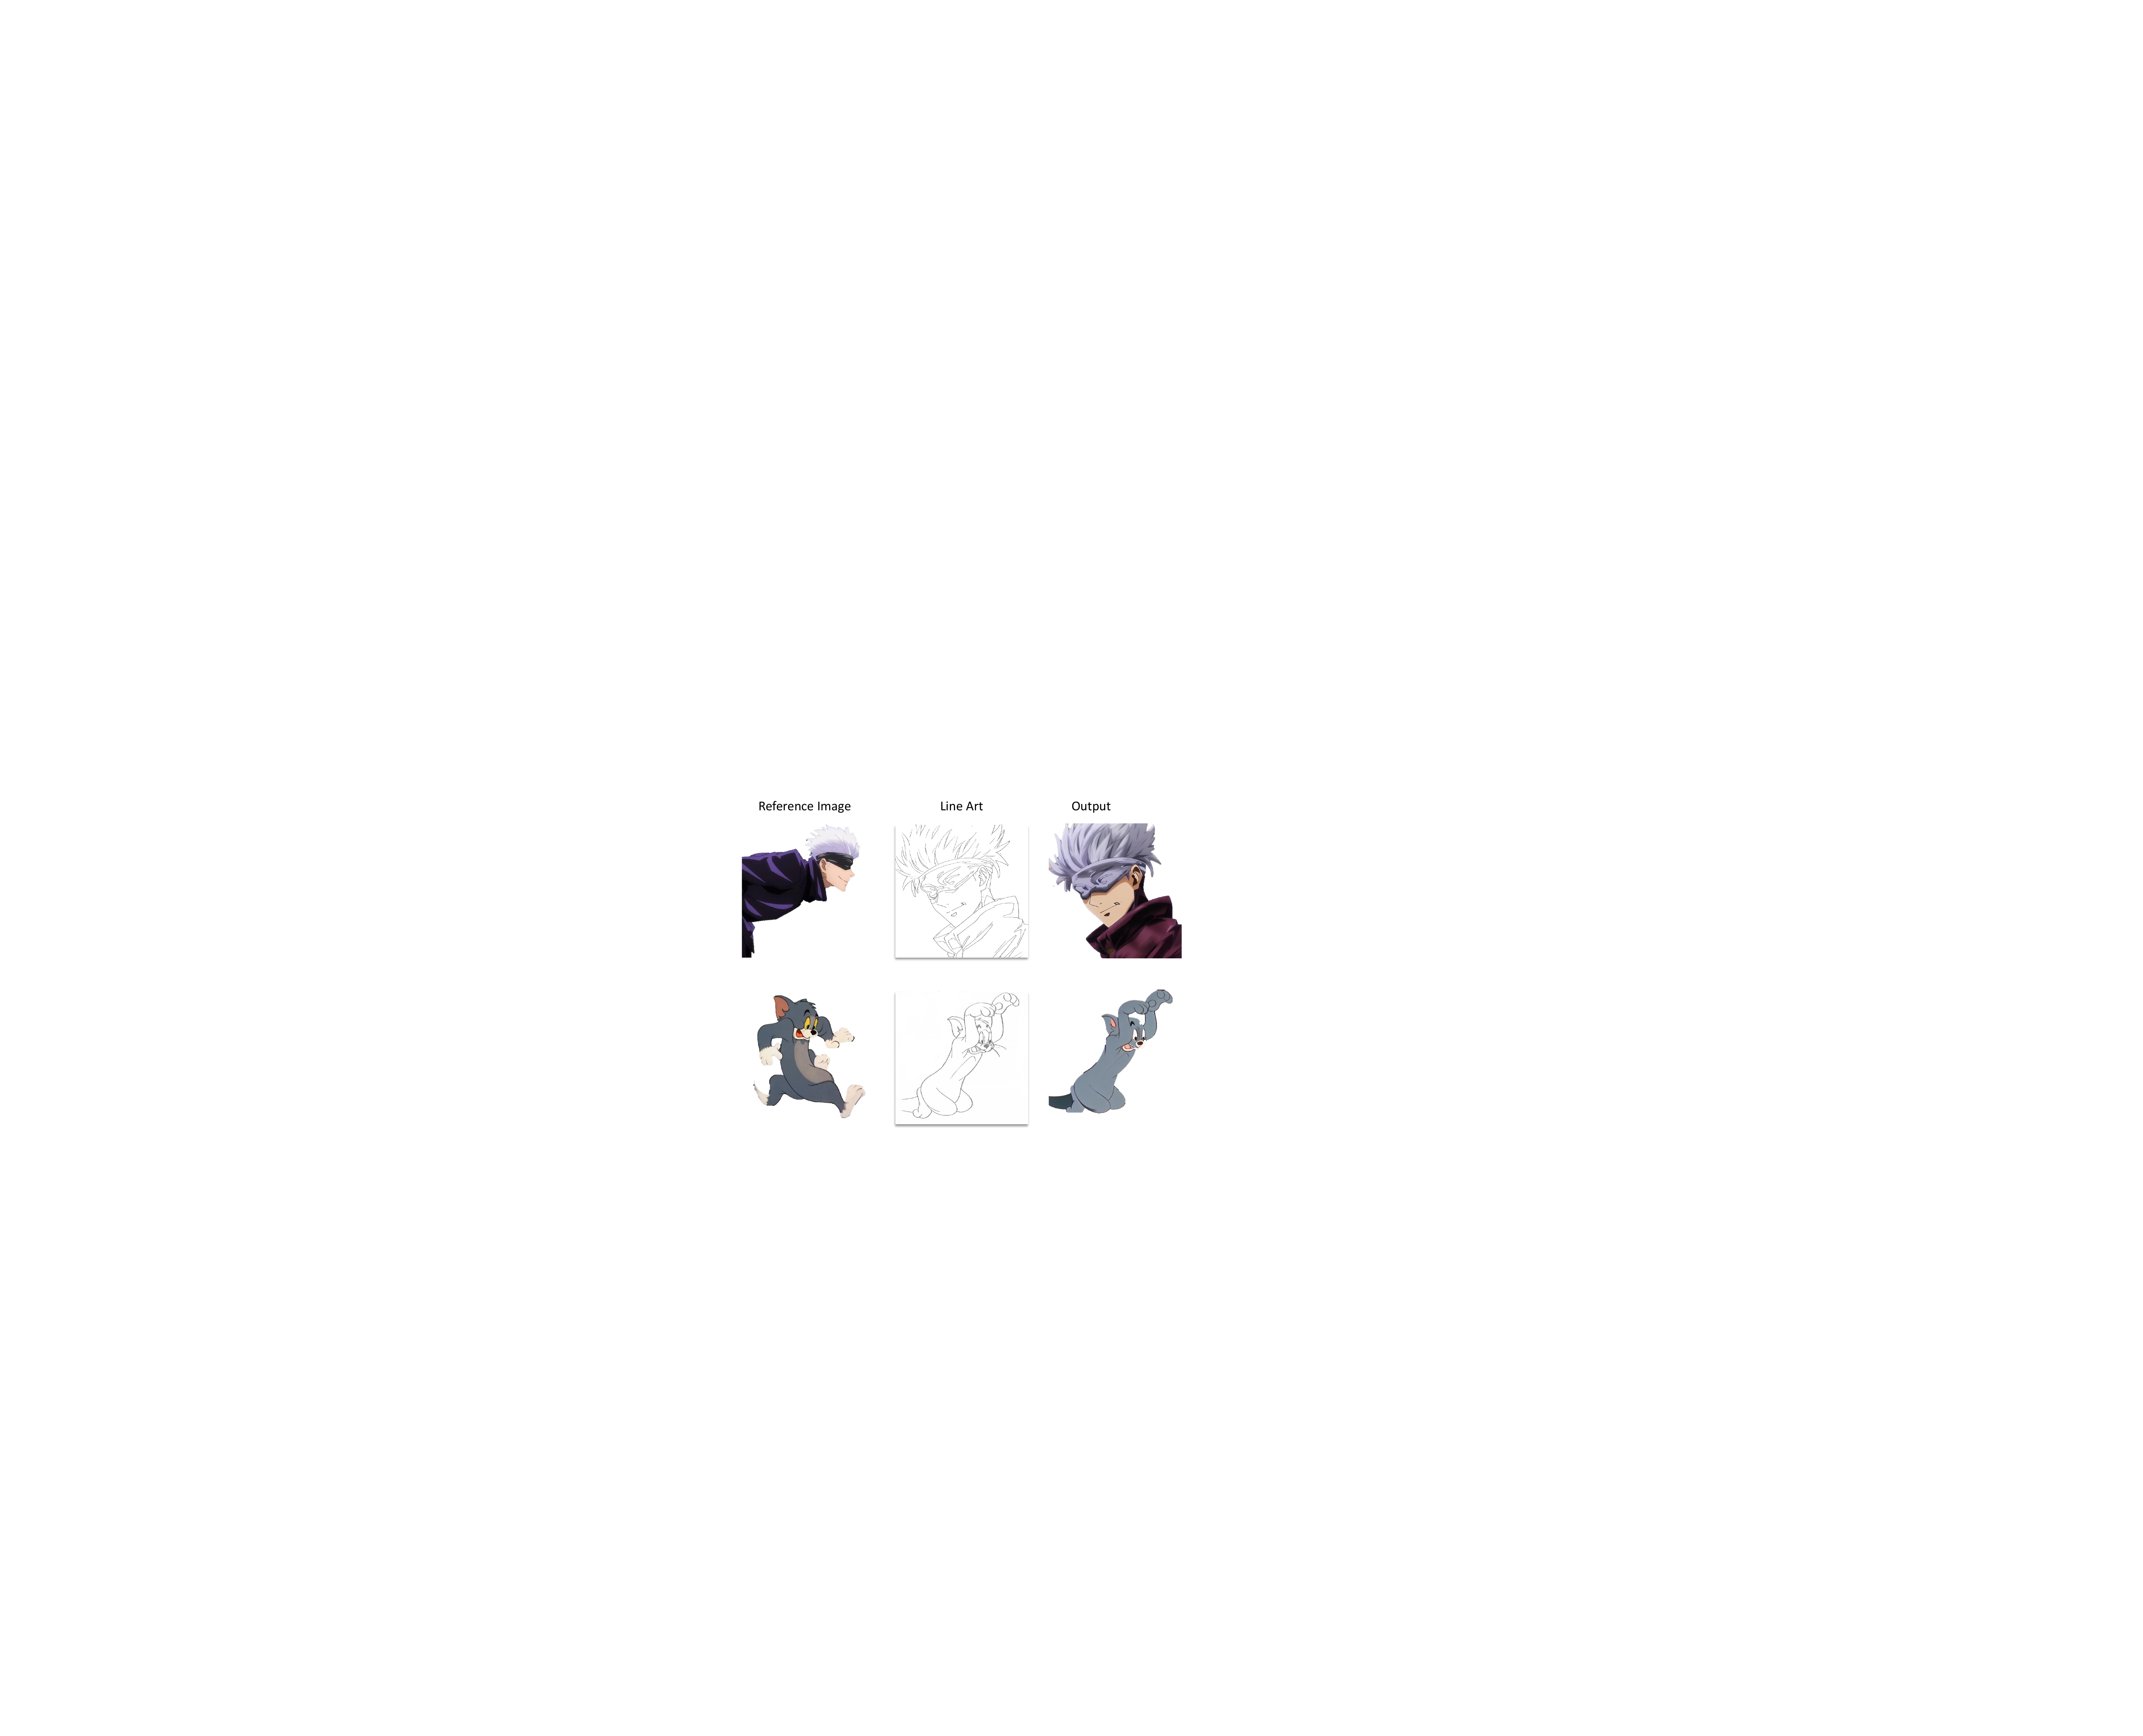}
    % \vspace{-0.35cm}
    \caption{\textbf{Performance of video colorization methods on non-Continuous line art.} We select LVCD for experiments because the line art conditioned generation code for ToonCrafter is not available.
    }
    \label{fig:supp1}
\end{figure}
We find that video line art colorization models like these work well only for continuous and small variations in line art. As shown in~\cref{fig:supp1}, when provided with a significantly different reference image and line art, these models fail to produce effective colorization. This limitation requires users to upload continuous line art sequences between the reference and target frames, which is impractical for single-image colorization.

\begin{figure}[t]
    \centering
    \includegraphics[width=1\linewidth]{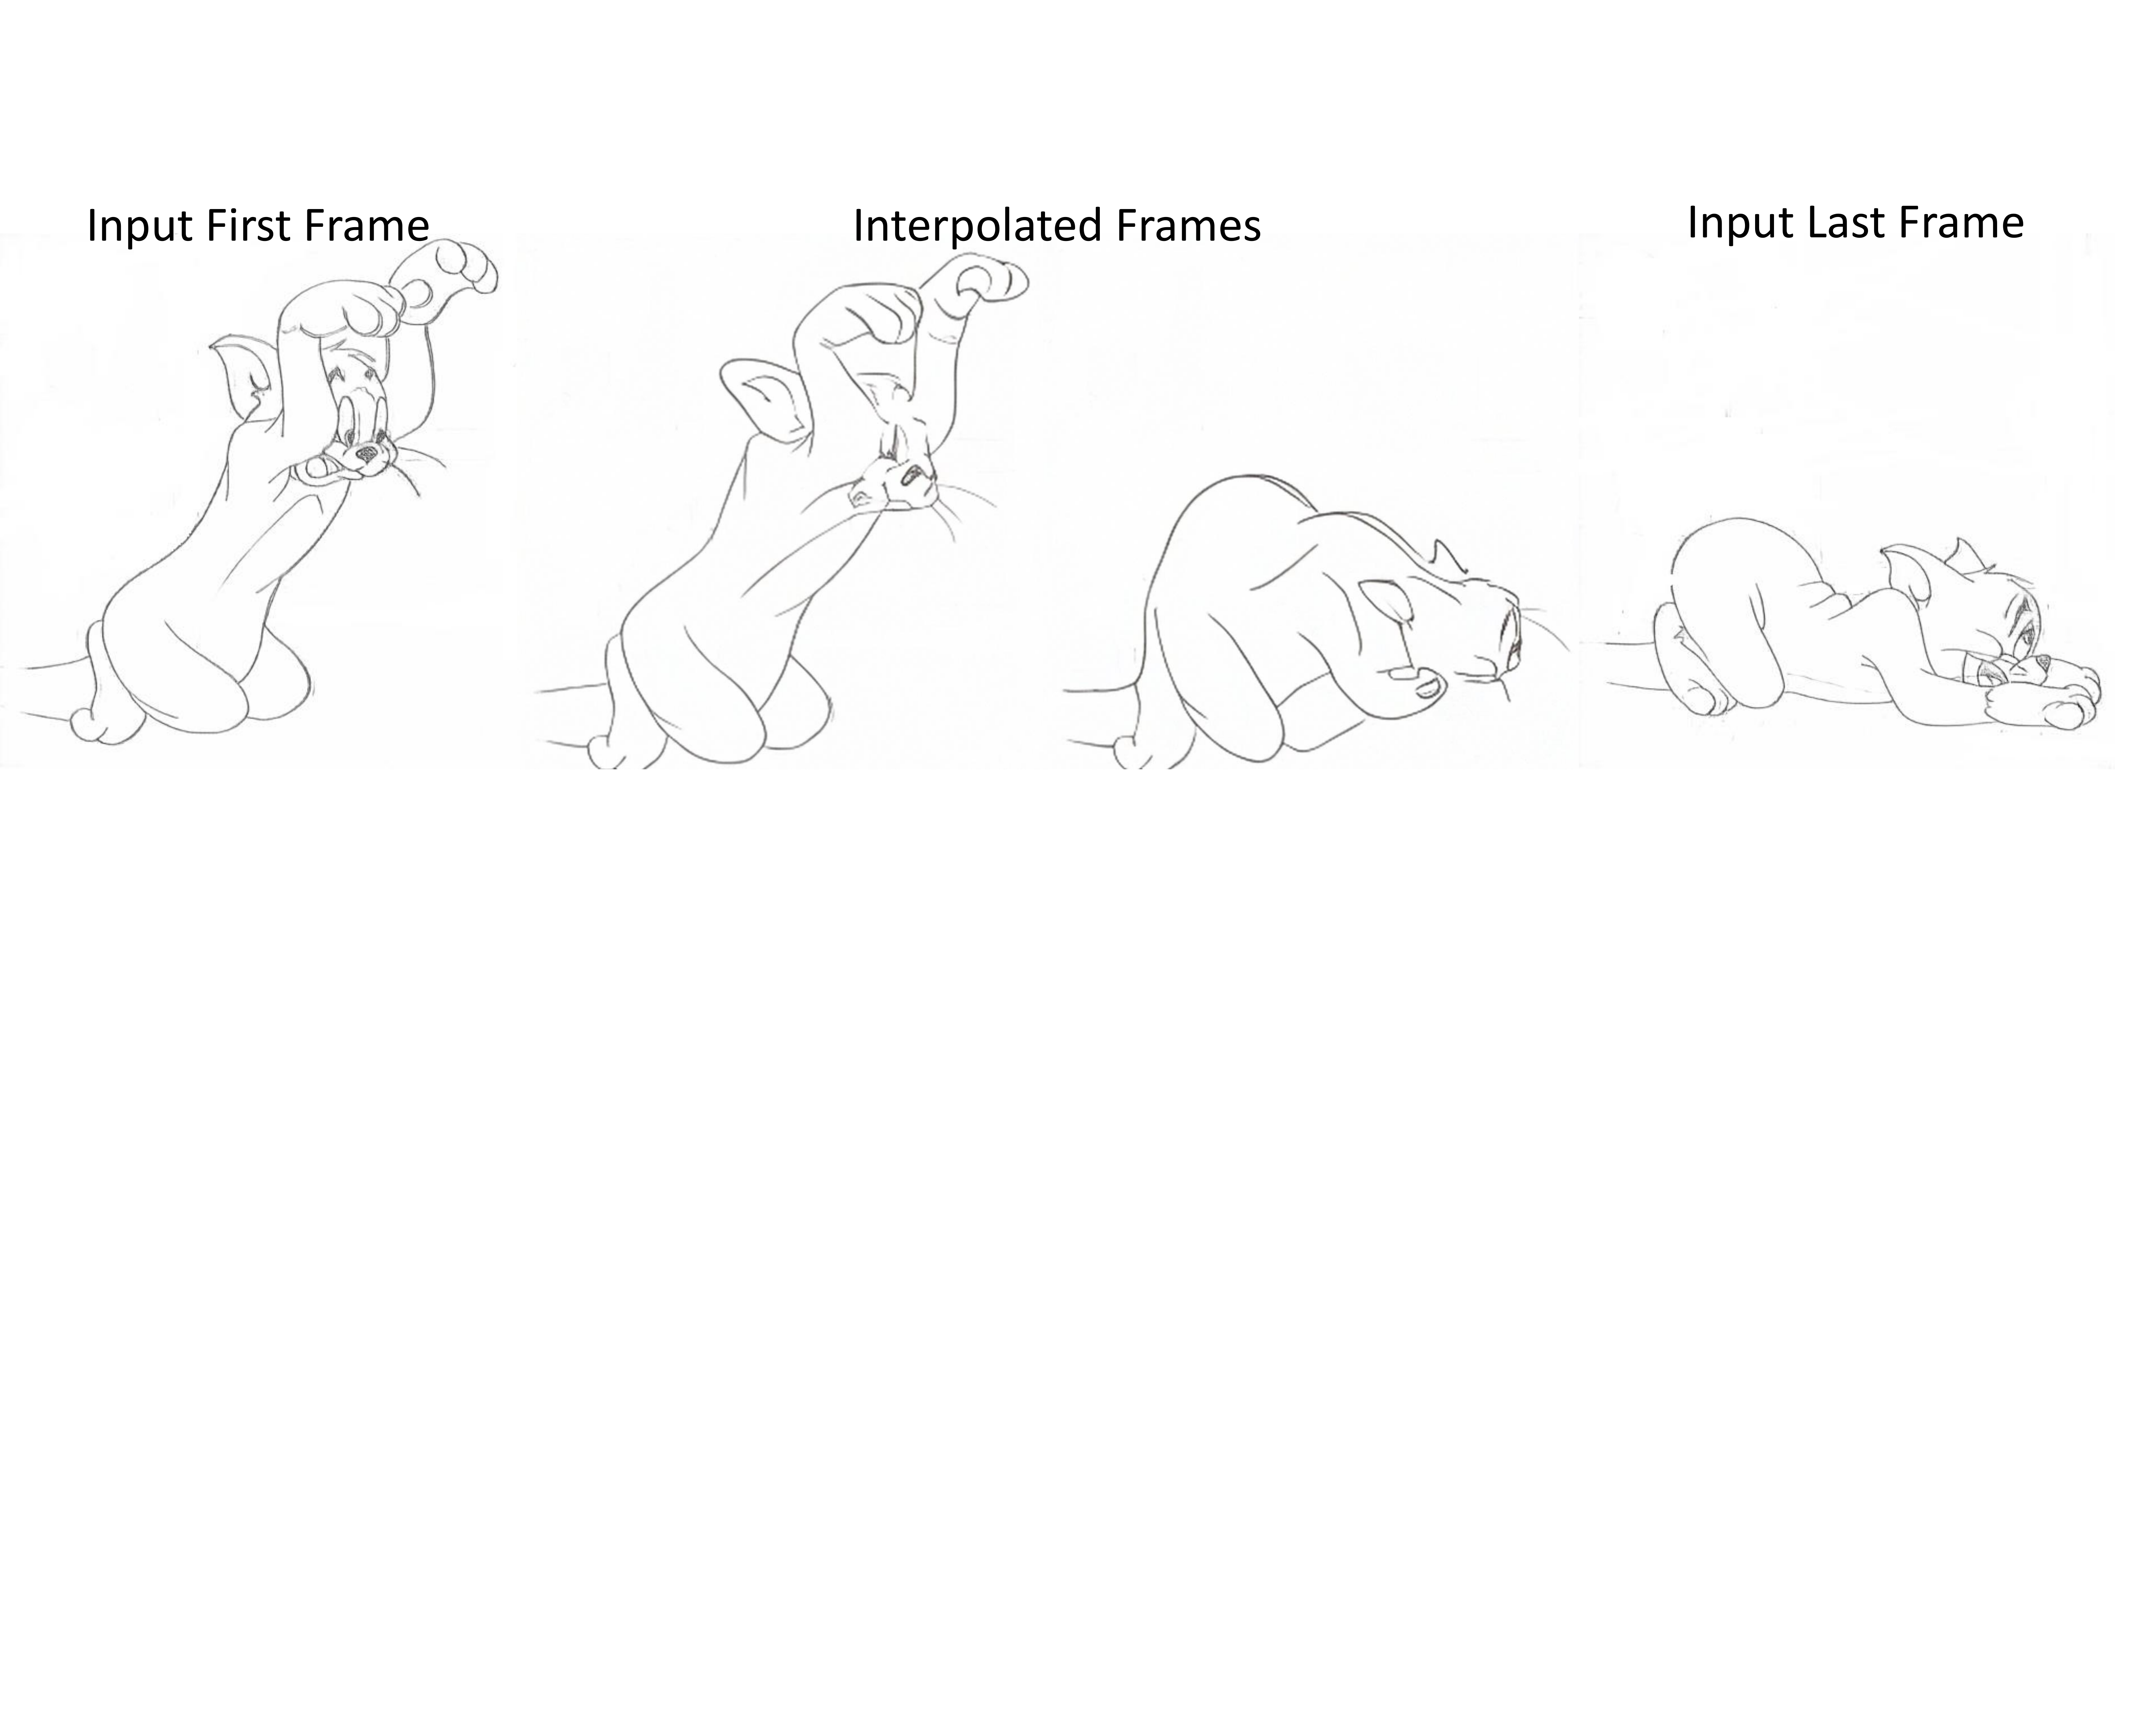}
    % \vspace{-0.35cm}
    \caption{\textbf{Line art interpolation results.}
    }
    \label{fig:inter}
\end{figure}
One possible solution is to generate intermediate line art via interpolation to pass reference information to the target frame. However, as illustrated in~\cref{fig:inter}, the current interpolation capabilities of video models have limitations. When there are large changes between the start and end frames, the generated interpolations lack consistency.
\begin{figure}[t]
    \centering
    \includegraphics[width=1\linewidth]{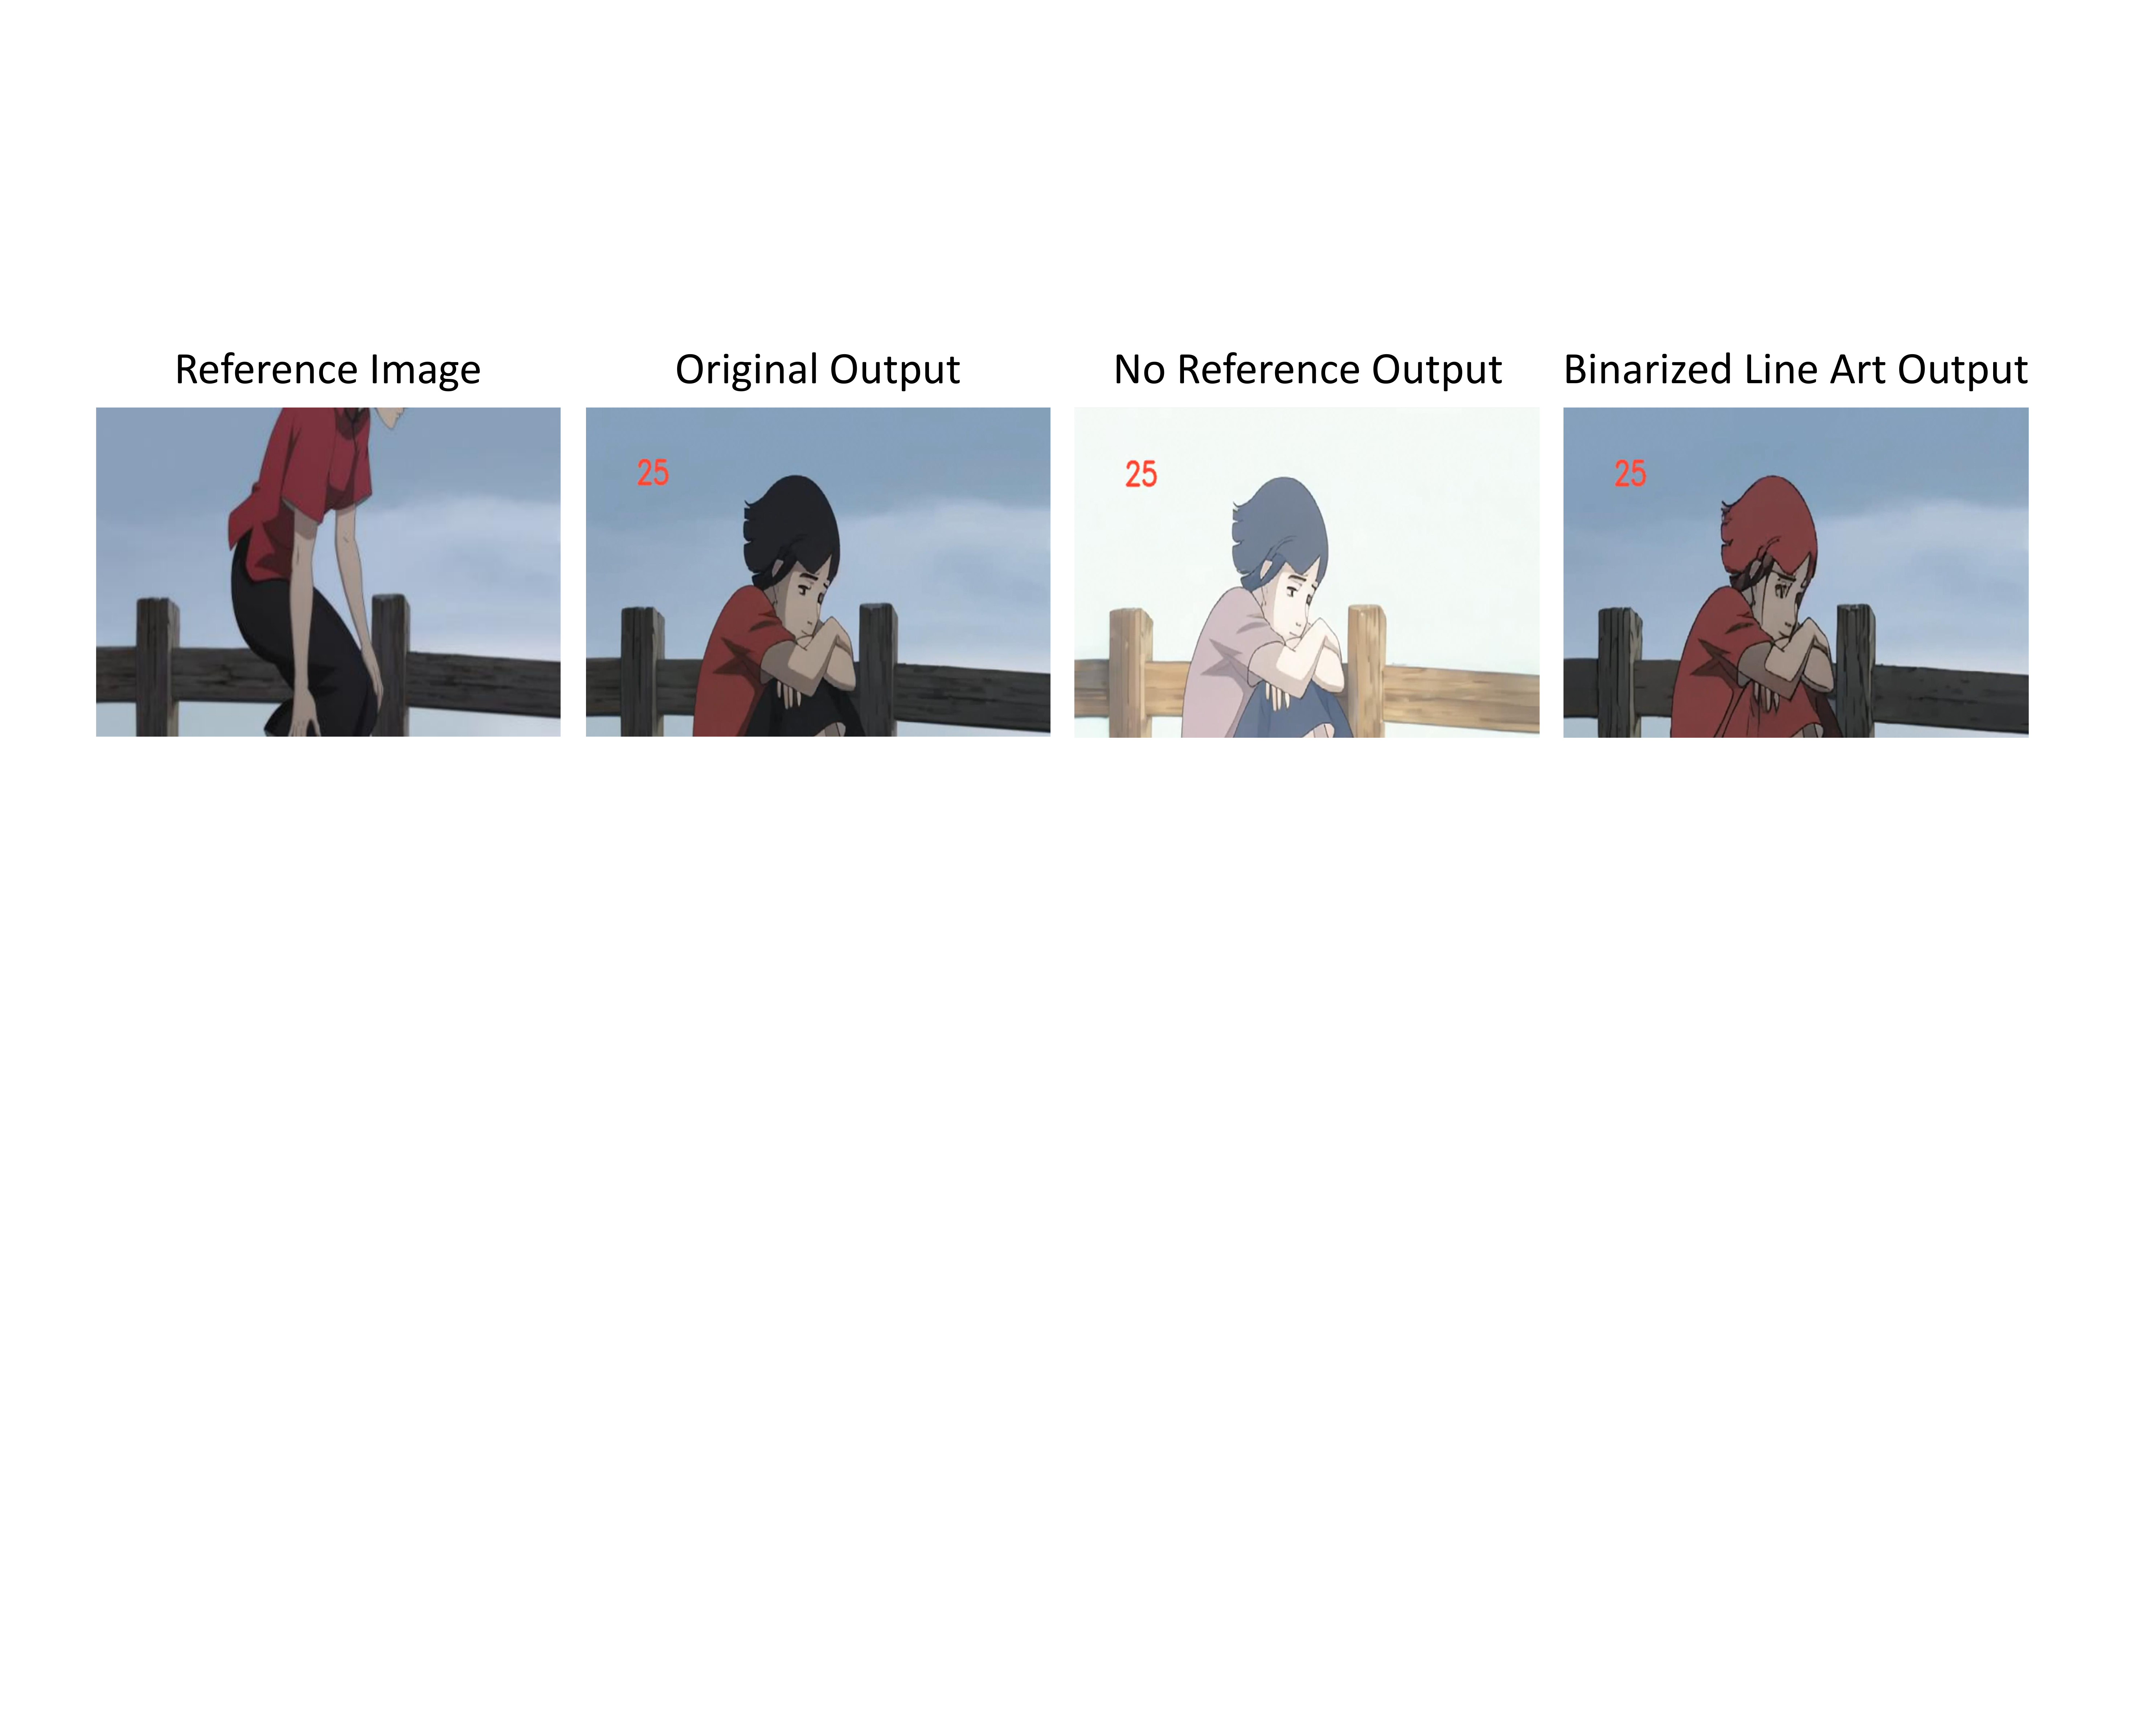}
    % \vspace{-0.35cm}
    \caption{\textbf{Visualization of GT leakage.} The `original output' represents the results from the paper. However, we find that when the reference image is empty, the model still generates outputs partially resembling the ground truth, as shown in `No Reference Output.' Moreover, setting low-value background regions in grayscale sketches to zero severely degrades the colorization quality.
    }
    \label{fig:gt}
\end{figure}
We also observe a color leakage issue with LVCD. As shown in~\cref{fig:gt}, when given non-binarized sketches, LVCD produces colorized results resembling the ground truth, even when the reference image is empty. This occurs due to the presence of low-value background regions that are invisible to the human eye (while the line art is represented as white with value 1, the background is nearly black, close to 0.) The network learns to map these subtle values to colors, causing ground truth leakage. Setting these low-value regions to zero eliminates the leakage, but it significantly degrades the colorization quality.

In contrast, \method~does not suffer from these issues. During training, we set low-value background areas in grayscale sketches to zero to avoid ground truth leakage. By incorporating effective training strategies and explicitly injecting correspondence information, \method~achieves precise matching, enabling accurate colorization even when there are large variations between the reference image and the line art.

\subsection{Analysis of RefOnly}
\begin{figure}[t]
    \centering
    \includegraphics[width=1\linewidth]{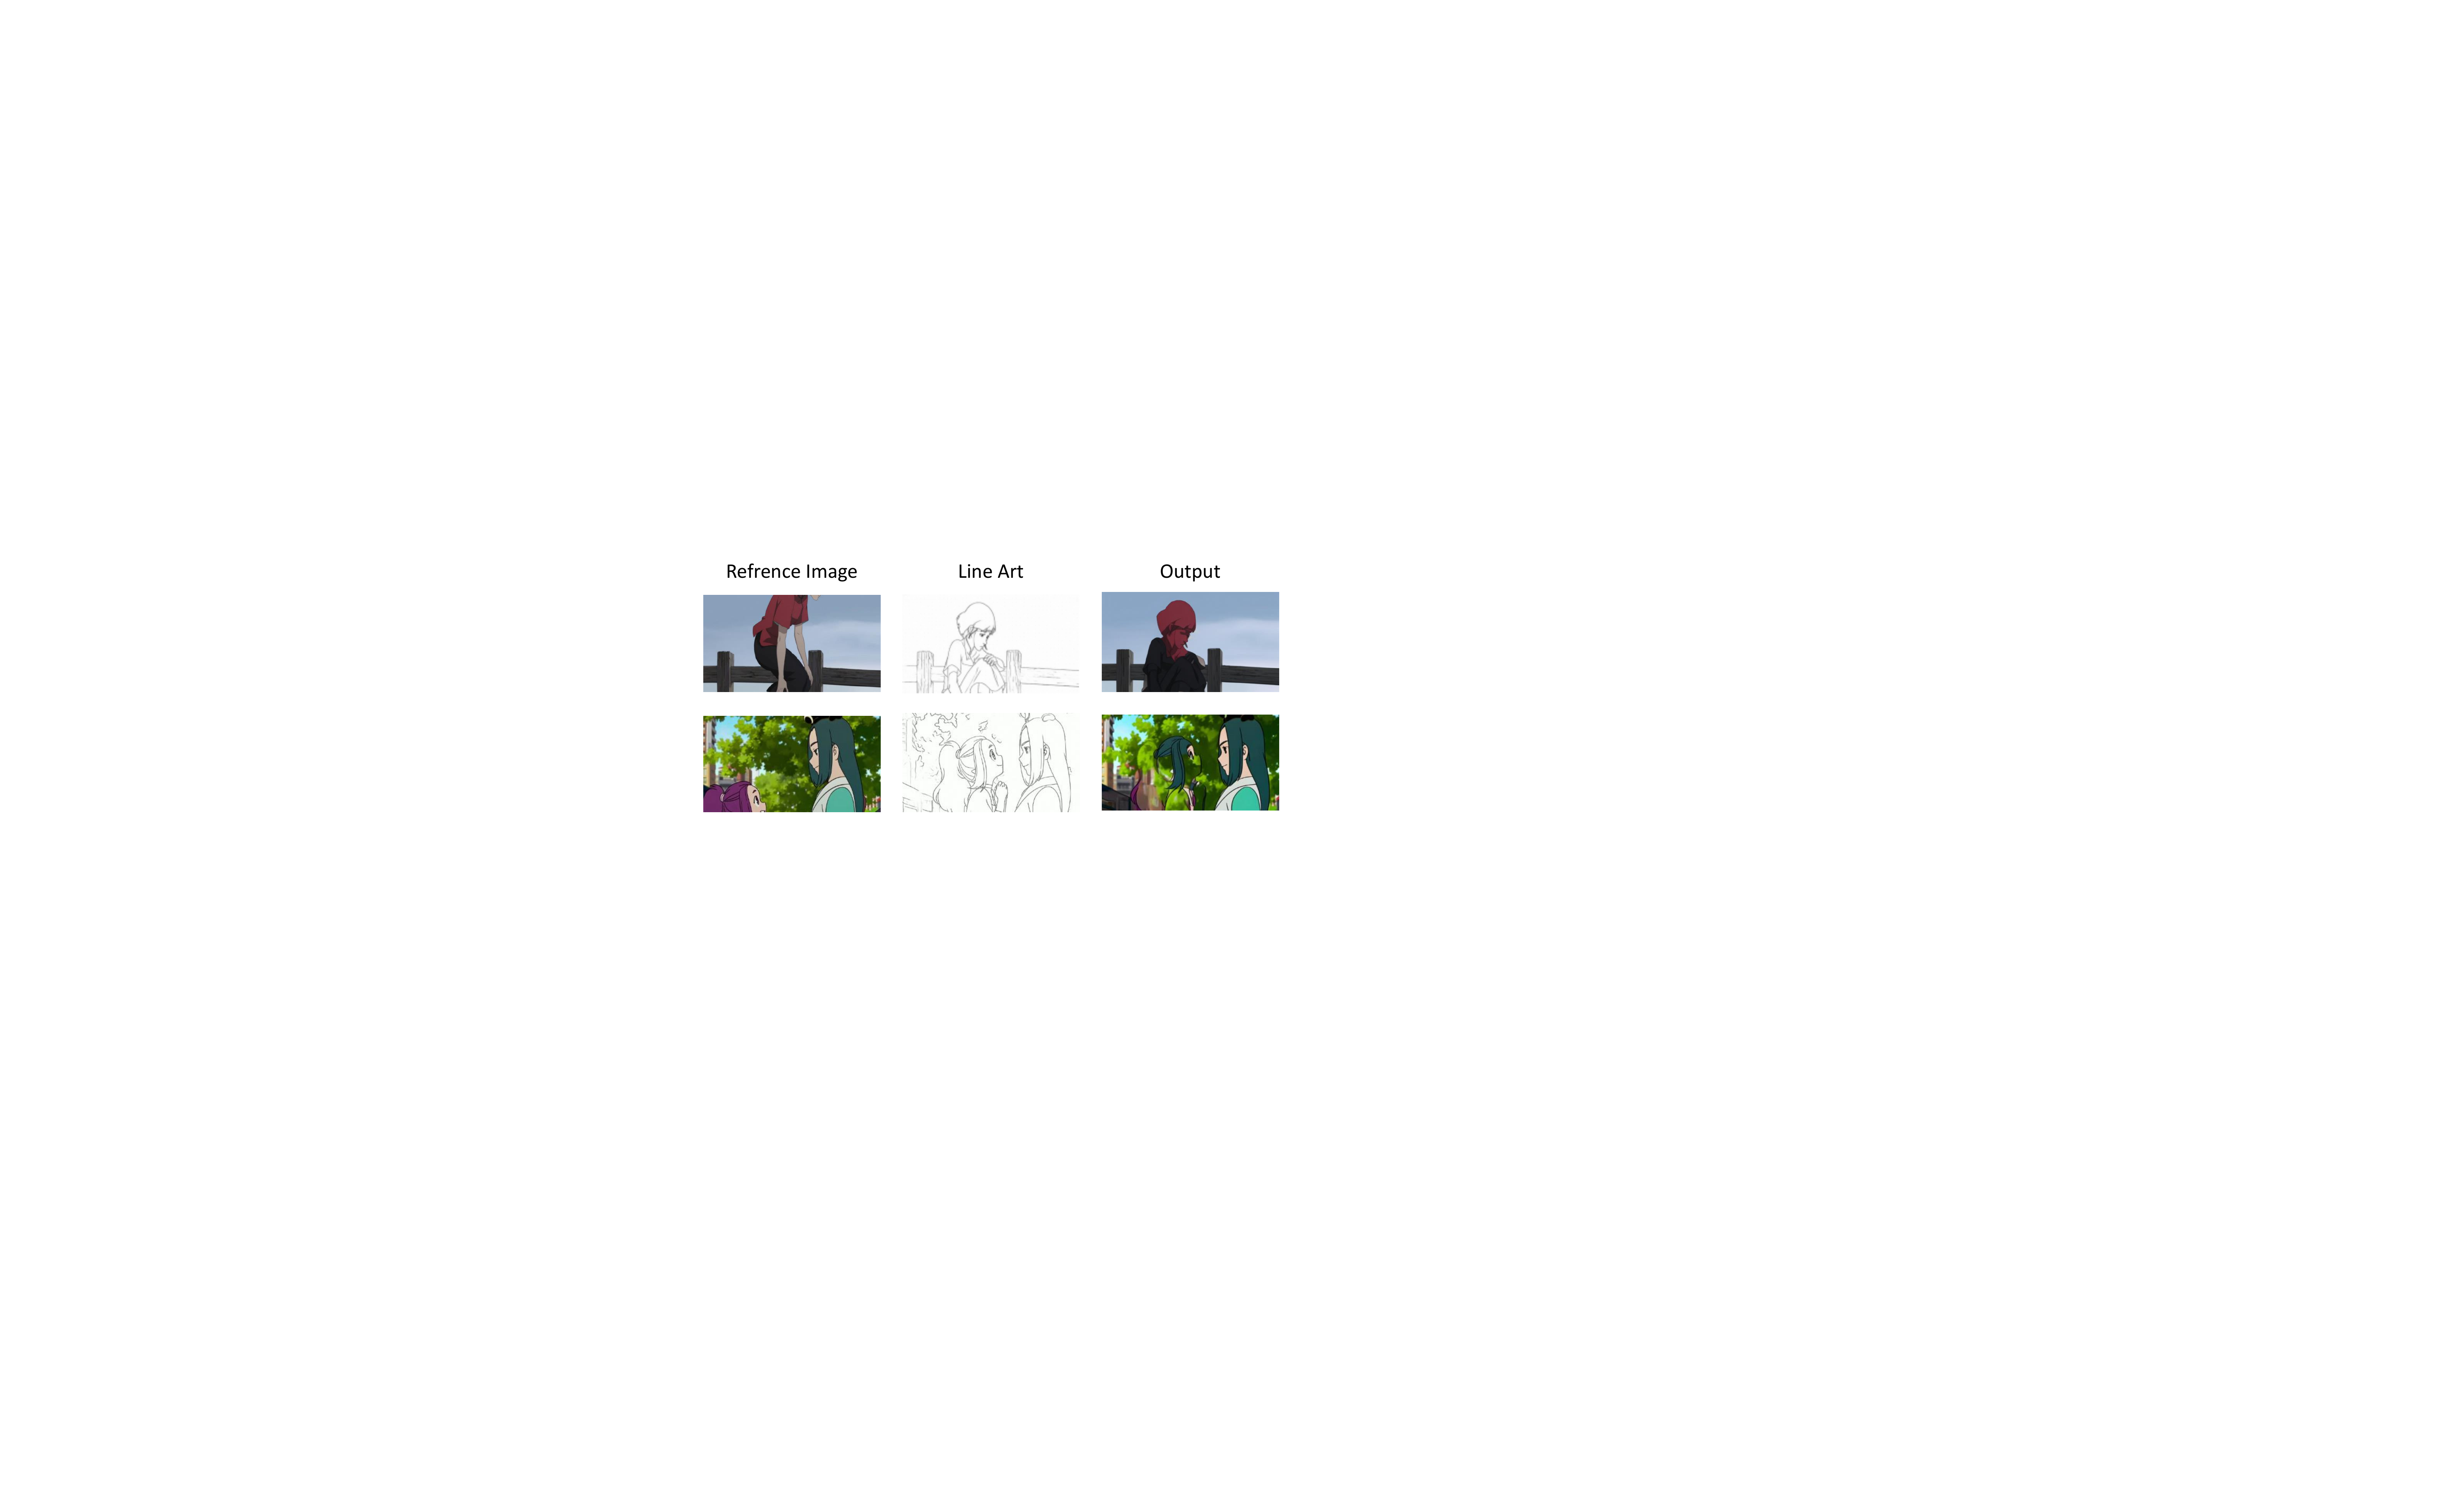}
    % \vspace{-0.35cm}
    \caption{\textbf{Visualization of RefOnly.}
    }
    \label{fig:ref}
\end{figure}
Another potential solution is to combine RefOnly with ControlNet~\cite{zhang2023adding}. As shown in~\cref{fig:ref}, similar to LVCD, a simple RefNet primarily maps the colors of the reference image onto the line art based on approximate spatial distribution, lacking precise matching capabilities.
\section{User Study and Benchmark}
\subsection{User study}
\begin{figure}[t]
    \centering
    \includegraphics[width=1\linewidth]{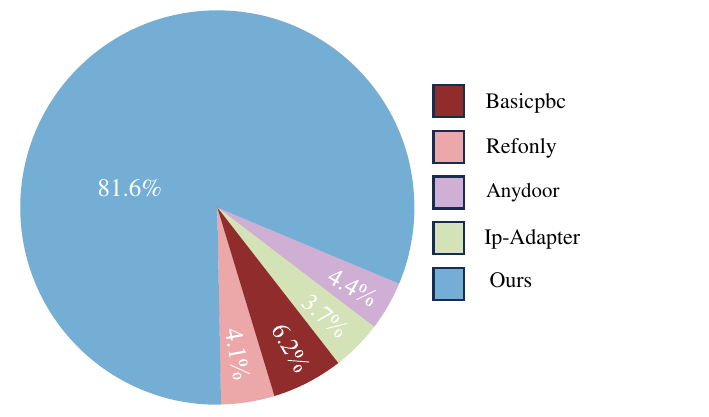}
    % \vspace{-0.35cm}
    \caption{\textbf{User study results.}
    }
    \label{fig:user}
\end{figure}
To further compare all methods, we also conduct a user study. Specifically, we select 40 pairs of reference images and line art for automatic colorization. We invite twenty participants, and each is asked to choose the method that produces the highest quality and most accurate color matching. 
As shown in~\cref{fig:user}, our method demonstrates a clear advantage over the others.
\subsection{Visual illustration of our benchmark}
\begin{figure}[t]
    \centering
    \includegraphics[width=1\linewidth]{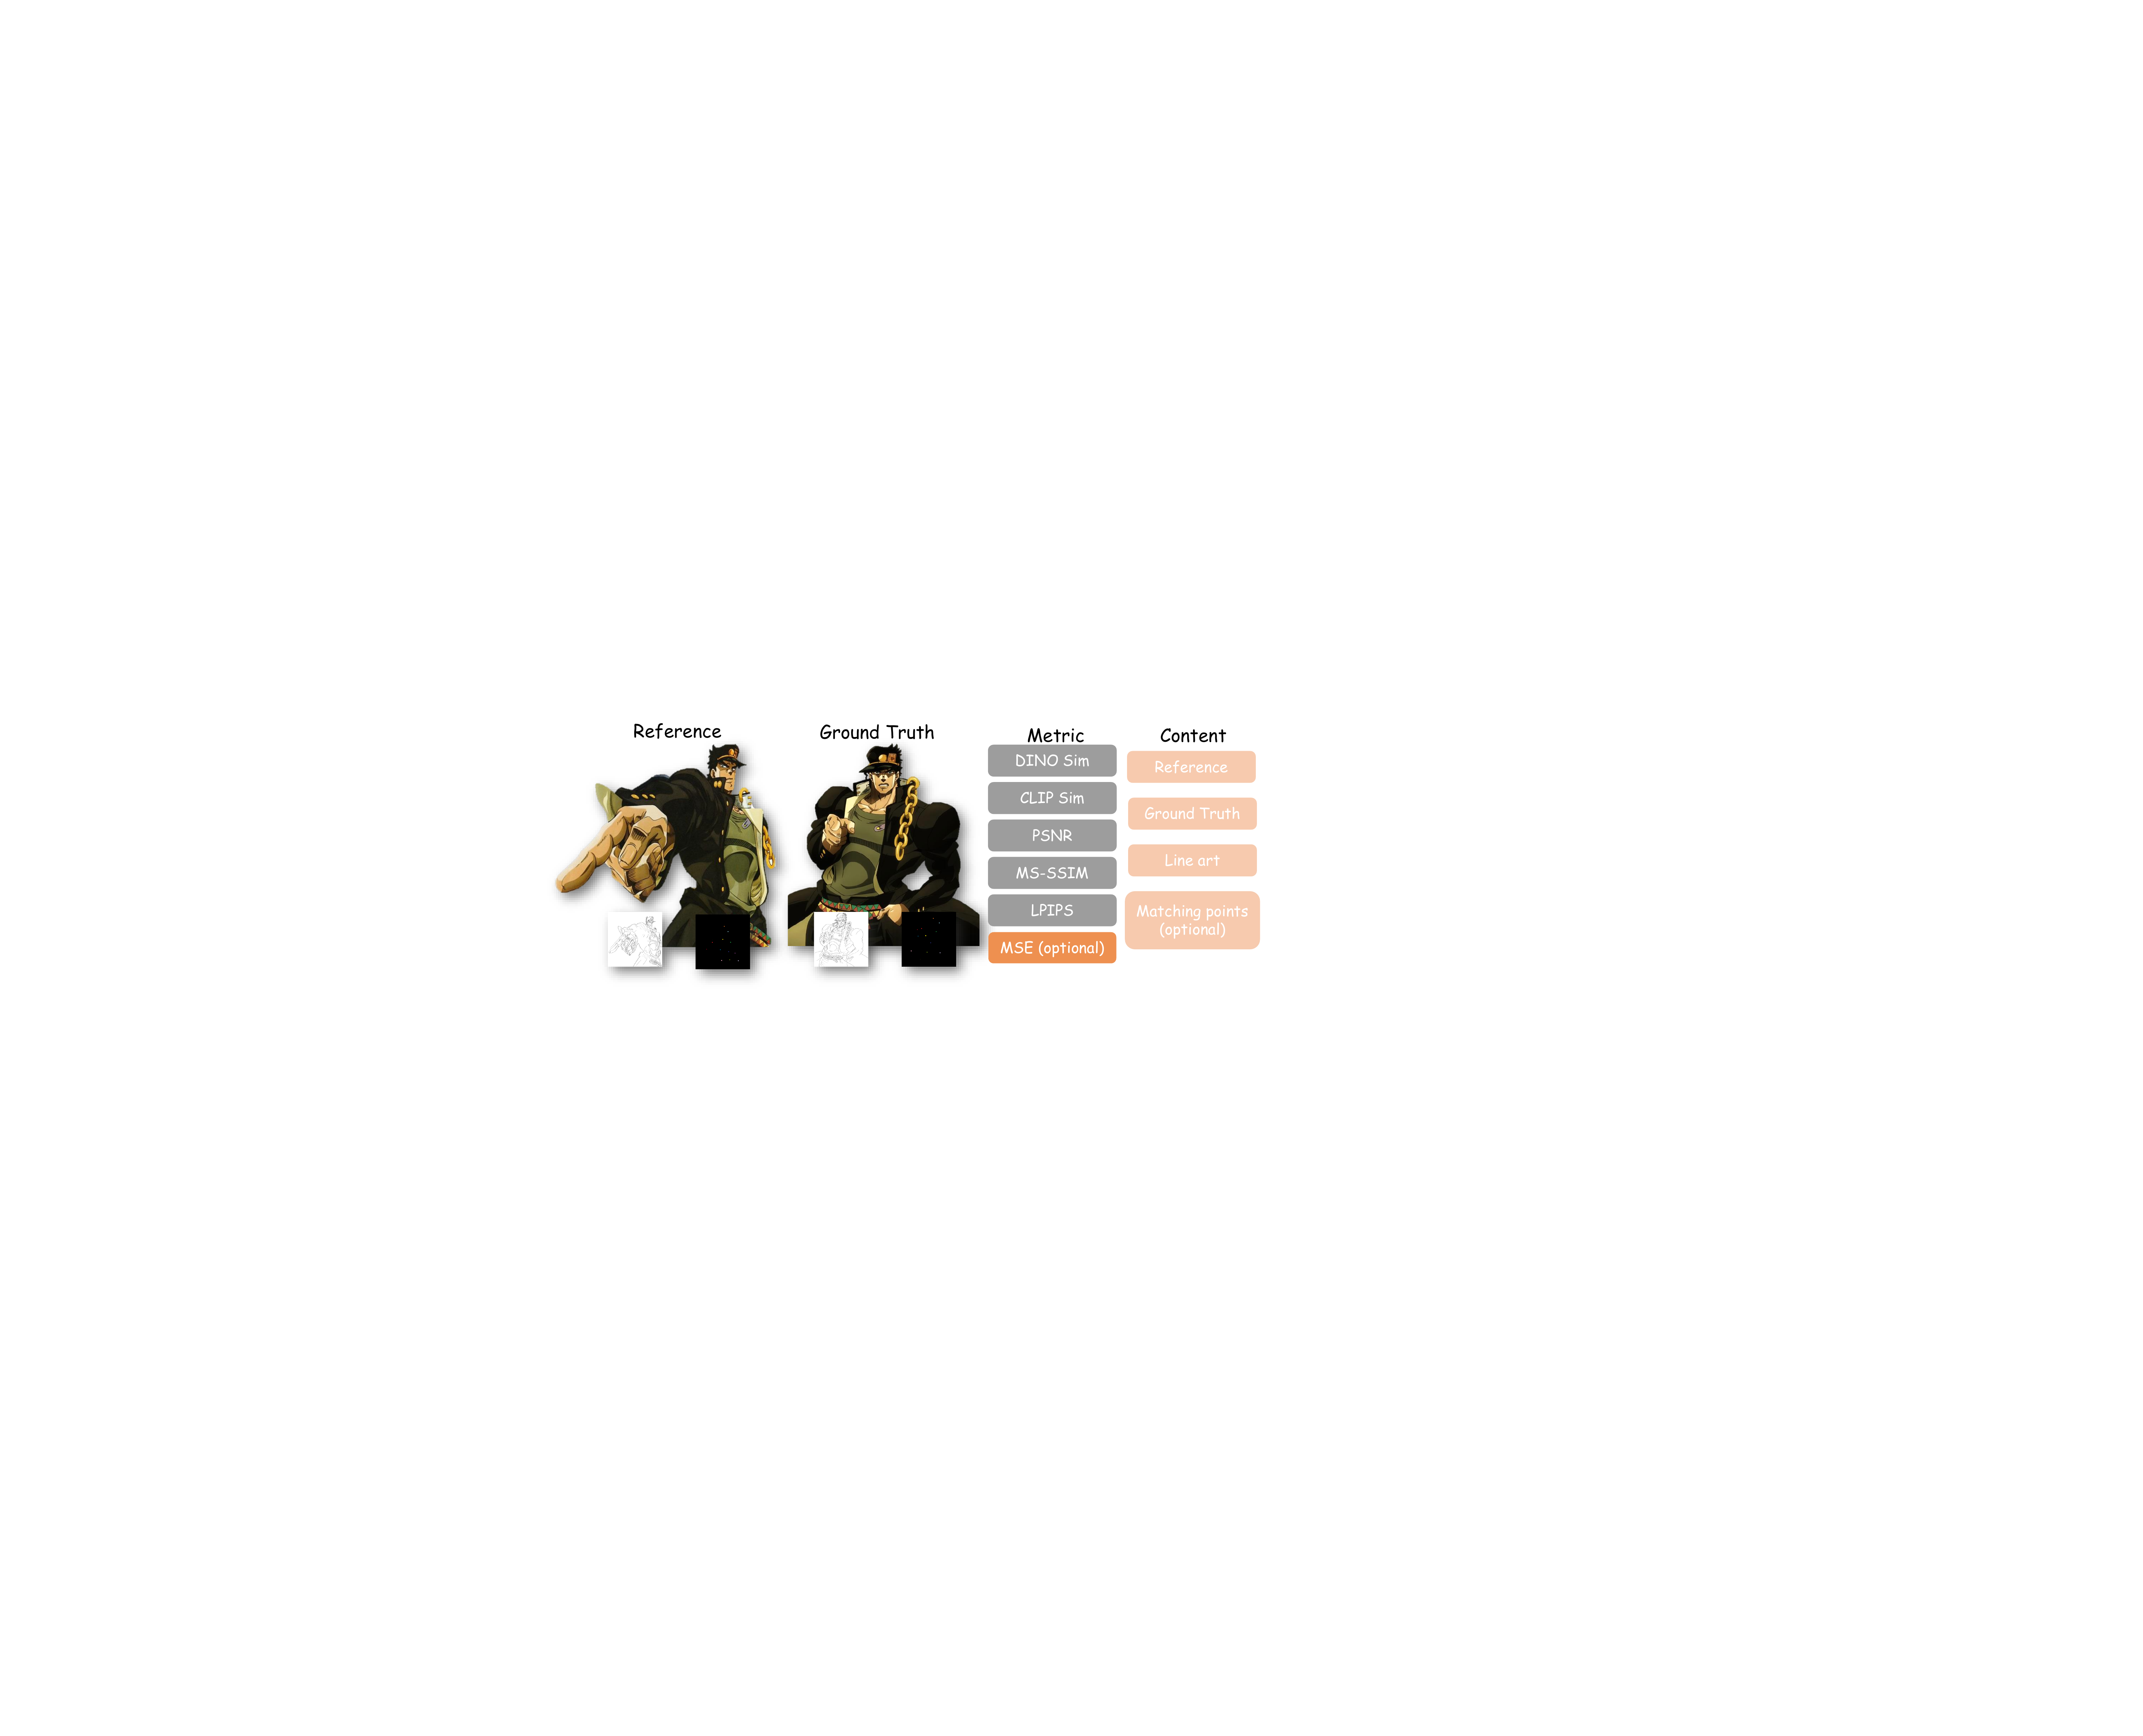}
    % \vspace{-0.35cm}
    \caption{\textbf{Illustration of constructed benchmark.}
    }
    \label{fig:bench}
\end{figure}
To provide a clearer explanation of the benchmark we constructed, we have selected an example for visualization. 
As shown in~\cref{fig:bench}, the background of the selected image is removed to avoid affecting metric calculations. 
Notably, in addition to common metrics, we provide matching points to calculate pixel-level MSE, which is used to evaluate the fine details of the colorization.
\section{More Ablation Studies}
\subsection{Reference feature extractor}
% \noindent\textbf{Image feature extractor.}
\begin{figure*}[t]
    \centering
    \includegraphics[width=1\linewidth]{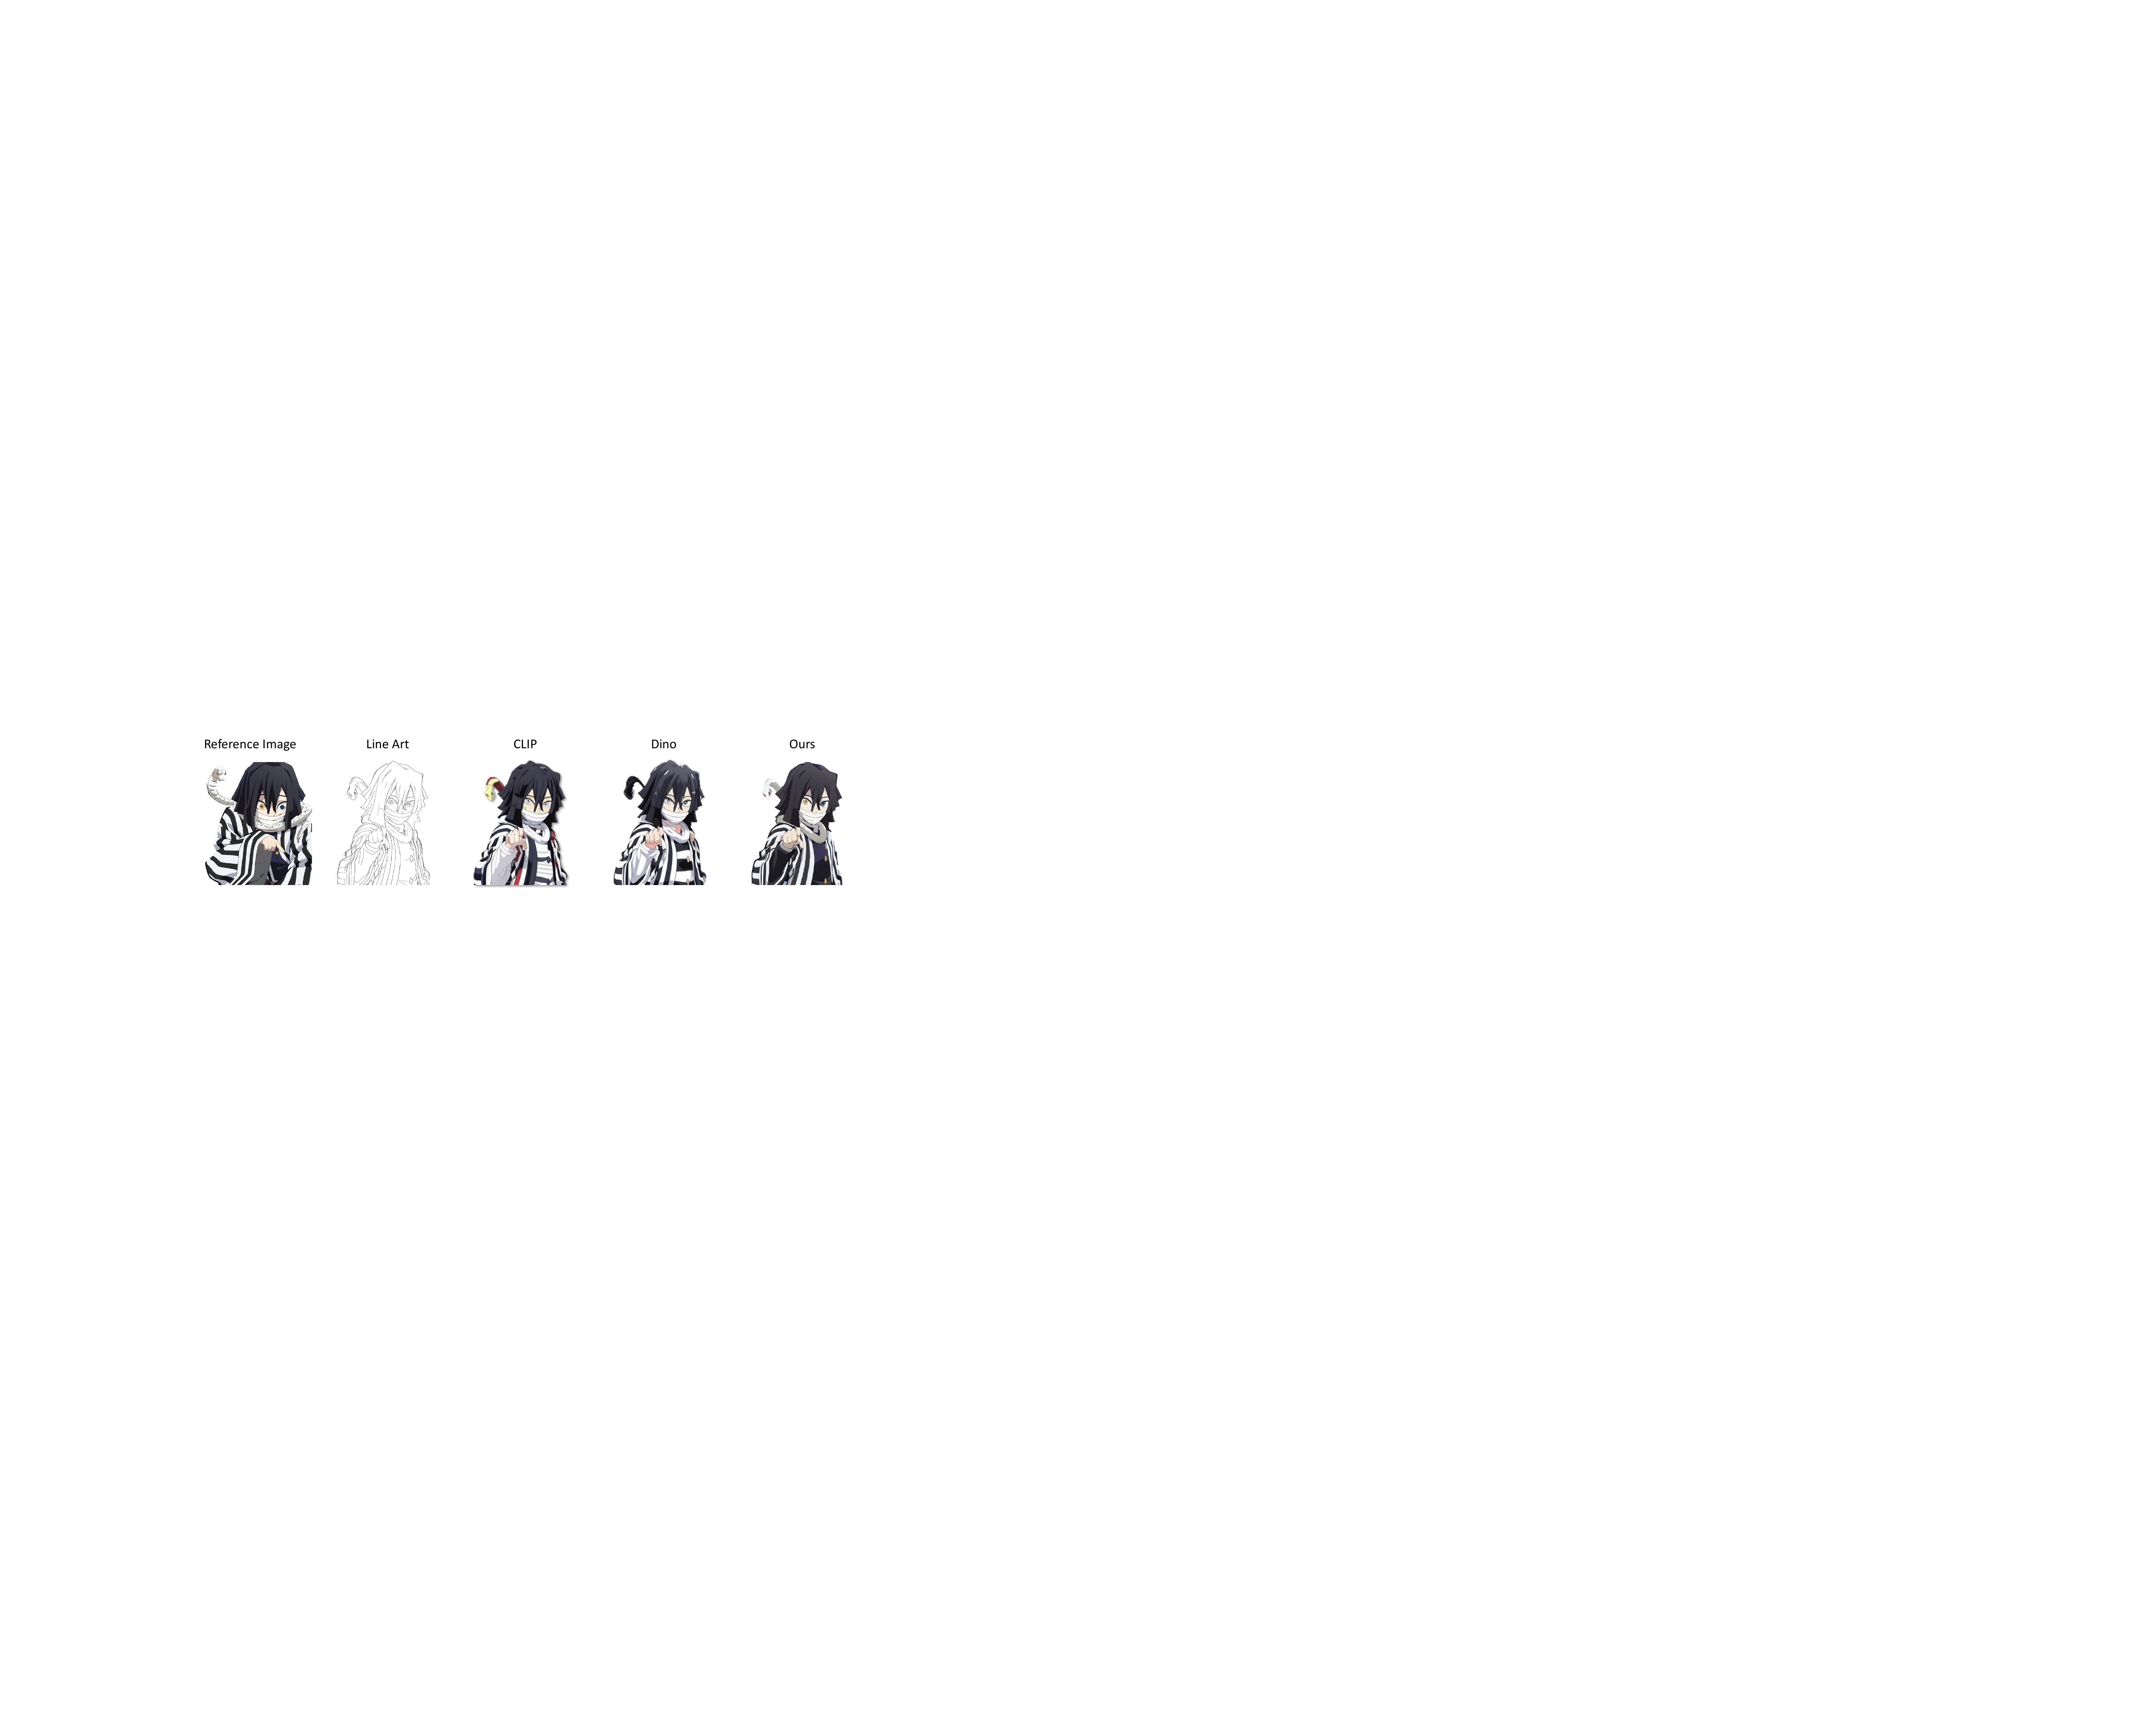}
    % \vspace{-0.35cm}
    \caption{\textbf{Comparison of different image feature extractors.}
    }
    \label{fig:image}
\end{figure*}
\method~employs a dual-branch U-Net to extract image features from the reference image and the target image, respectively. To validate the effectiveness of the Reference U-Net structure in learning matching capabilities, we replace the reference U-Net with DINO and CLIP image encoders, injecting $16 \times 16$ patch tokens within the cross-attention layers, while keeping all other training settings identical. The experiments are conducted using the same dataset and experimental settings. All training strategies are applied in the same way.
As shown in~\cref{fig:image}, compared with the Reference U-Net, using CLIP or DINO as the encoder results in weaker handling of fine details.
\begin{table*}[h]
    \centering
    \small
    \caption{
        \textbf{Ablation of patch shuffle.} Note that each model in the table inherits from the previous one, with an increased number of shuffled patches used for training.
    }
    \label{tab:patch}
    % \vspace{-8pt}
    \SetTblrInner{rowsep=1.2pt}      % Row space.
    \SetTblrInner{colsep=8.0pt}      % Col space.
    \begin{tblr}{
        cells={halign=c,valign=m},   % Text alignment for all cells.
        column{1}={halign=l},        % Text alignment for the first column.
        hline{1,2,6,8}={1-6}{},       % Horizontal lines.
        hline{1,8}={1.0pt},          % Horizontal line width.
        vline{2}={1-7}{},         % Vertical lines.
    }
    Number of shuffled patches                            & DINO $\uparrow$ & CLIP $\uparrow$ &  PSNR $\uparrow$ & MS-SSIM $\uparrow$ & LPIPS $\downarrow$ \\
    $2\times2$                  & 63.91               & 84.75              & 18.02           & 0.912              & 0.27  \\
    $4\times4$                & 64.42               & 85.23              & 18.44           & 0.924             & 0.25  \\
    $8\times8$ & 65.13               & 85.87              & 18.77           & 0.935            & 0.25  \\
    $16\times16$  & 66.69               & 86.49             & 19.24& 0.943             & 0.24  \\
    $32\times32$                             & \textbf{67.12}      & \textbf{86.93}     & \underline{19.72}  & \underline{0.952}     & \textbf{0.23} \\
    $64\times64$ & \textbf\underline{67.09}  & \underline{86.86} & \textbf{19.88} & \textbf{0.954} & \textbf{0.23}
    \end{tblr}
    % \vspace{-5pt}
\end{table*}
\subsection{Progressive patch shuffle}
The purpose of our patch shuffle strategy is to disrupt the structural information in the reference image, preventing the model from learning a simple offset to perform colorization. Instead, we want the model to develop a finer-level matching ability. Thus, how to effectively disrupt the structure becomes a key question.
We find that using overly fine-grained shuffles during training (e.g., dividing the patches into $32\times32$ segments) makes it difficult for the model to converge. On the other hand, using a coarse shuffle (e.g., dividing into $2\times2$ patches) fails to adequately break down the structural information. Therefore, we adopt a coarse-to-fine learning scheme by progressively increasing the number of randomly shuffled patches. Specifically, we multiply the number of shuffled patches by four every 40k steps. 

As shown in~\cref{tab:patch}, we apply patch shuffle to the base model without additional training strategies or point guidance. With an increasing number of shuffled patches, the model’s performance improves consistently until the difference between $32\times32$ and $64\times64$ becomes negligible. Therefore, we ultimately set the shuffled patch size to $32\times32$.

\section{More Results}
\begin{figure*}[!h]
    \centering
    \includegraphics[width=0.75\linewidth]{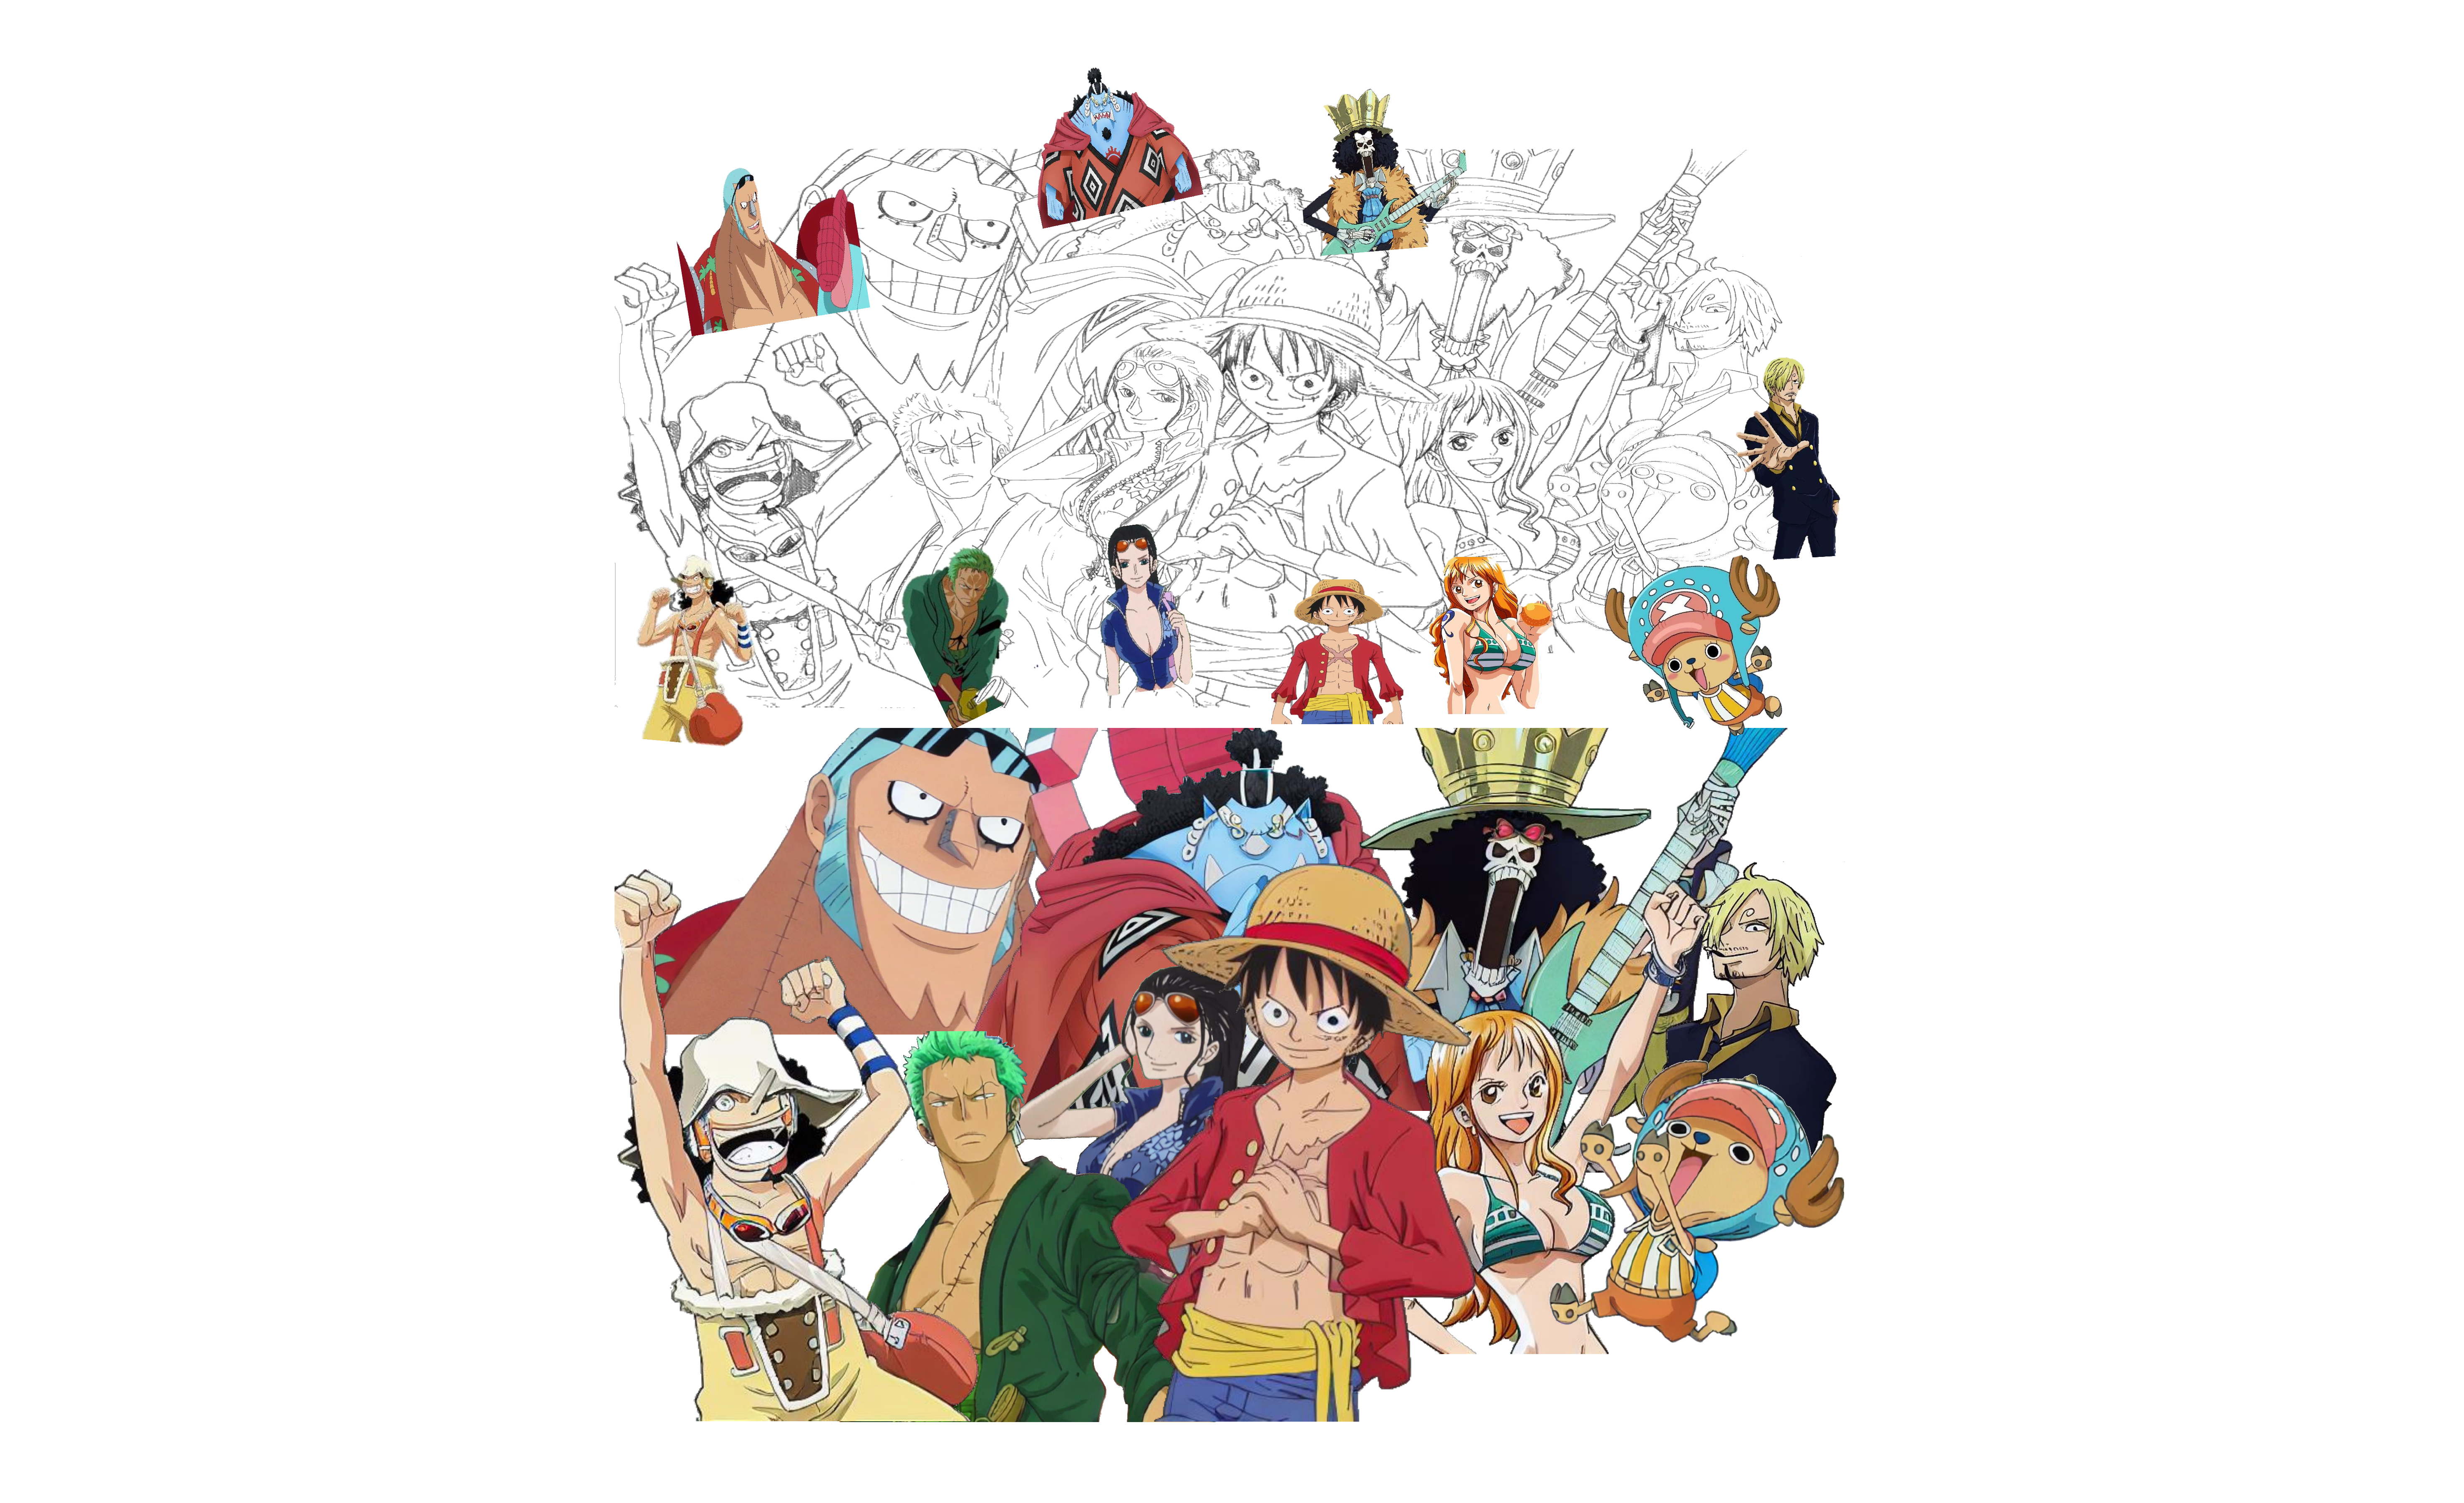}
    % \vspace{-0.35cm}
    \caption{\textbf{Colorization results for \textit{One Piece} characters.}
    }
    \label{fig:one}
\end{figure*}

\begin{figure*}[t]
    \centering
    \includegraphics[width=0.75\linewidth]{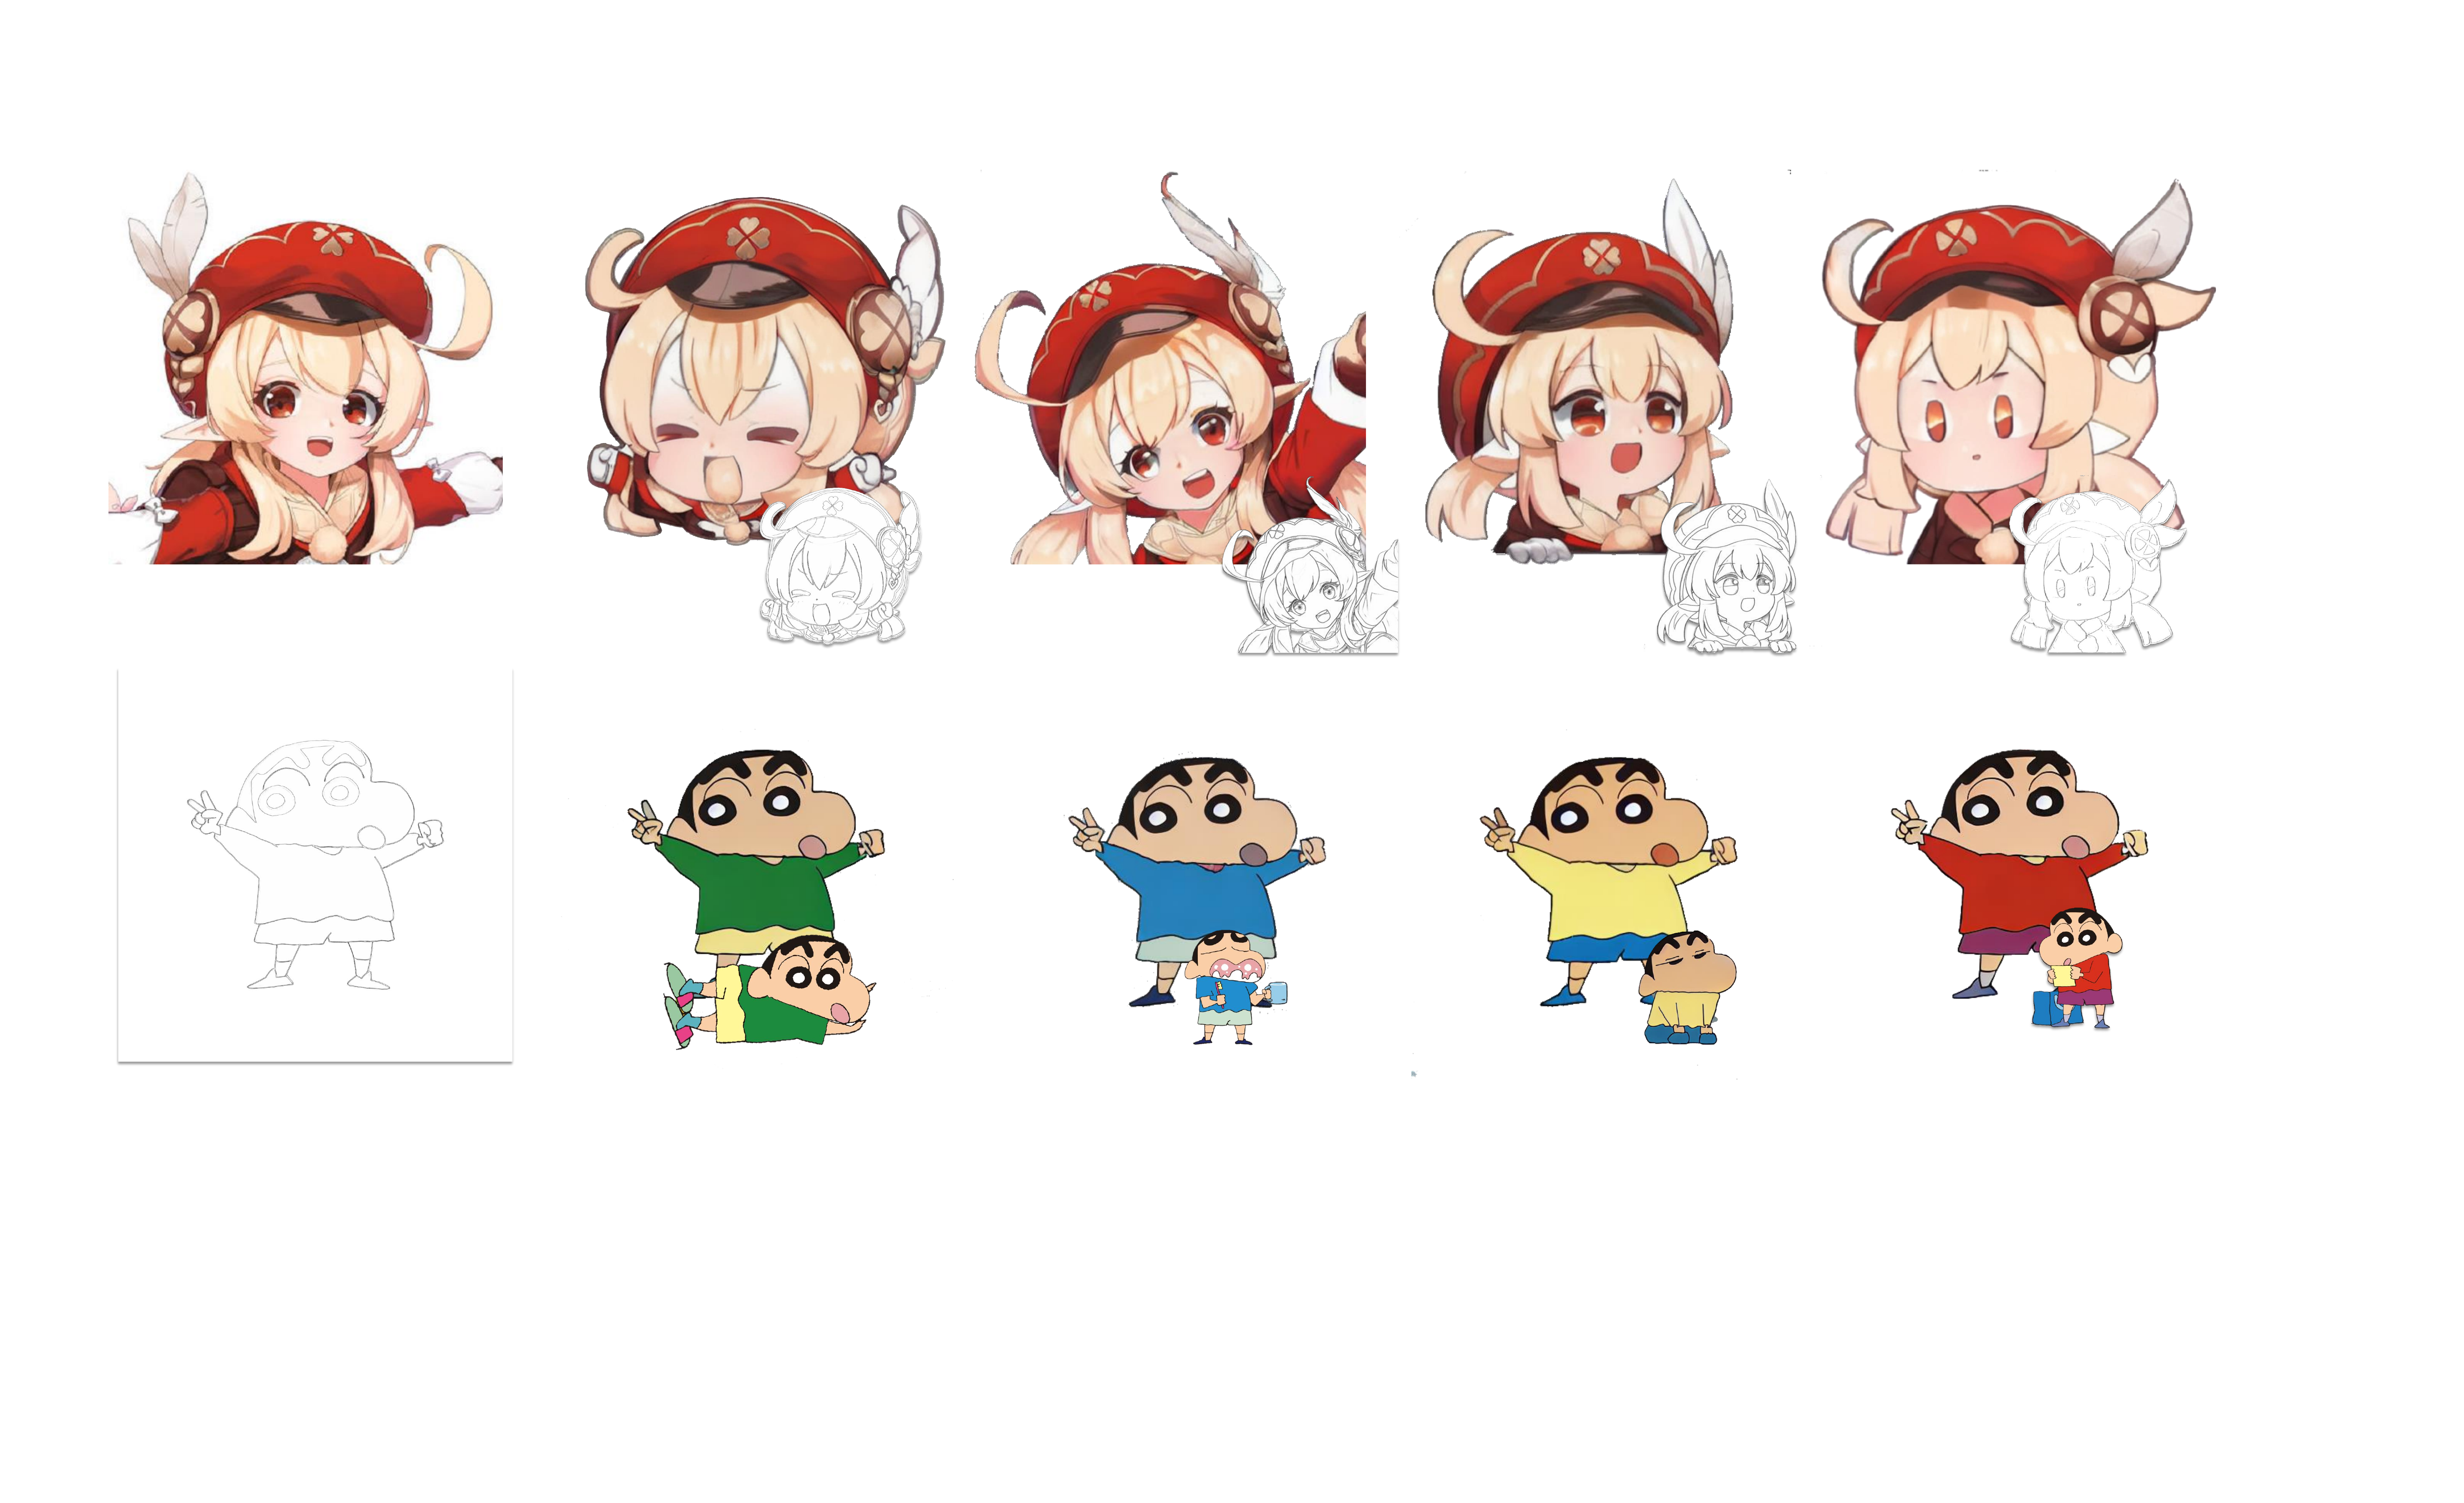}
    % \vspace{-0.35cm}
    \caption{\textbf{More visualization results.} One reference to colorize multiple line art images in row one; multiple references to colorize the same sketch in row two.
    }
    \label{fig:multi_one}
\end{figure*}
To further demonstrate the precise matching capability of \method, we provide additional visual results. As shown in~\cref{fig:one}, we colorize all characters from the manga \textit{One Piece}. As shown in~\cref{fig:multi_one}, we use the same reference with different line art images in row one and the same line art with different references in row two. The results show that our method exhibits strong robustness.
